# Supplementary material for: Intention Aware Robot Crowd Navigation with Attention-Based Interaction Graph
Source: arXiv:2203.01821 source file (2023-04-24)
Supplement: Supplementary file 1 [file Appendix.tex]

\section{Appendix}
\label{sec:append}
Not provided in the submitted version
